# Supplementary material for: $\text{R}^2$-Bench: Benchmarking the Robustness of Referring Perception Models under Perturbations
Source: arXiv:2403.04924 source file (2024-03-07)
Supplement: Supplementary file 1 [file appendix.tex]

\tabrisrefcocoevalsupp{t}
\tabrisrefcocotestasupp{t}
\tabrisrefcocotestbsupp{t}
\tabrisrefcocopevalsupp{t}
\tabrisrefcocoptestasupp{t}
\tabrisrefcocoptestbsupp{t}
\tabrisrefcocogevalsupp{t}
\tabrisrefcocogtestasupp{t}
\tabrisrefcocogtestbsupp{t}
\tabdavissupp{t}
\tabrvosPfull{t}
\tabavsP{t}
\tabrvosdyn{t}
\tabvosdyn{t}
